# Supplementary material for: From Attack Success to Attack Severity: Counterfactual Memory Attacks on LLM Agents
Source: arXiv:2609.34132 source file (2026-09-28)
Supplement: Supplementary file 1 [file appendix_contents.tex]

% Appendix-only contents, populated automatically by sectioning commands.
\pdfbookmark[0]{Appendix Contents}{appendix.contents}
\section*{Appendix Contents}
\vspace{0.8em}
\makeatletter
\begingroup
  \setcounter{tocdepth}{2}
  \renewcommand{\l@section}[2]{%
    \addvspace{0.65em}%
    {\bfseries\@dottedtocline{1}{0em}{2em}{#1}{#2}}}
  \renewcommand{\l@subsection}[2]{%
    \@dottedtocline{2}{1.6em}{3em}{#1}{#2}}
  \@starttoc{apc}
\endgroup
% Retain hyperref's anchors while routing only appendix entries to this list.
\let\memharm@addcontentsline\addcontentsline
\renewcommand{\addcontentsline}[3]{%
  \ifnum\pdfstrcmp{#1}{toc}=0
    \memharm@addcontentsline{apc}{#2}{#3}%
  \else
    \memharm@addcontentsline{#1}{#2}{#3}%
  \fi}
\makeatother
\clearpage
